# Supplementary material for: Structural and electronic properties of solid molecular hydrogen from many-electron theories
Source: arXiv:2011.09529 source file (2020-11-18)
Supplement: Supplementary file 1 [file supp.pdf]

# Supplementary Information for “Structural and electronic properties of solid molecular hydrogen from many-electron theories”

Ke Liao\*

*Max Planck Institute for Solid State Research, Heisenbergstrasse 1, 70569 Stuttgart, Germany*

Tong Shen\*

*School of Physics, State Key Laboratory for Artificial Microstructure  
and Mesoscopic Physics, Peking University, 100871 Beijing, China*

Xin-Zheng Li

*School of Physics, State Key Laboratory for Artificial Microstructure  
and Mesoscopic Physics, Peking University, 100871 Beijing, China and  
Collaborative Innovation Centre of Quantum Matter, Peking University, 100871 Beijing, China*

Ali Alavi

*Max Planck Institute for Solid State Research, Heisenbergstrasse 1, 70569 Stuttgart, Germany and  
Department of Chemistry, University of Cambridge,  
Lensfield Road, Cambridge CB2 1EW, United Kingdom*

Andreas Grüneis<sup>†</sup>

*Institute for Theoretical Physics, Vienna University of Technology,  
Wiedner Hauptstrasse 8-10, 1040 Vienna, Austria*

---

\* These two authors contributed equally

<sup>†</sup> andreas.grueneis@tuwien.ac.at

# NUCLEAR FORCES FROM THE SECOND ORDER MØLLER-PLESSET THEORY USING A PLANE WAVE BASIS

## Theoretical Formulation

In this section, we briefly recapitulate the theoretical formulation of analytical gradients given by the second order Møller-Plesset theory (MP2), while focusing on the differences between using a nuclei-position dependent Gaussian basis and a nuclei-position independent plane wave basis. For the detailed derivations, we refer to [1, 2], in particular we follow the derivation from Ref. [2] closely.

Starting from the mean-field Hartree-Fock theory, the MP2 theory perturbatively adds some correlation effects to observables. For example, the total energy can be expressed as

$$E_{\text{MP2}} = E_{\text{HF}} + E_{\text{MP2}}^{\text{corr}}, \quad (1)$$

following which the total forces also consists of two parts

$$\mathbf{F} = \mathbf{F}_{\text{HF}} + \mathbf{F}_{\text{MP2}}^{\text{corr}}, \quad (2)$$

since the energy and force are related simply by the following expression

$$\mathbf{F} = -\frac{\partial E}{\partial \mathbf{R}}, \quad (3)$$

where  $\mathbf{R}$  is a vector of all the nuclear positions.

For a closed-shell system, the MP2 correlation energy can be expressed as

$$E_{\text{MP2}}^{\text{corr}} = \sum_{ijab} t_{ij}^{ab} \langle ij|ab \rangle, \quad (4)$$

$$t_{ij}^{ab} = \frac{(2 \langle ij|ab \rangle - \langle ij|ba \rangle)}{\varepsilon_i + \varepsilon_j - \varepsilon_a - \varepsilon_b}, \quad (5)$$

where the indices  $i, j$  and  $a, b$  refer to the occupied and unoccupied Hartree-Fock (HF) orbitals, respectively, and the  $\varepsilon_{i,j,a,b}$  are the corresponding orbital energies. Here we adopt the convention to use  $i, j, k, l, \dots$ ,  $a, b, c, d, \dots$  and  $p, q, r, s, \dots$  as occupied, unoccupied and general orbital indices, respectively. The orbitals are linear combinations of the underlying plane wave basis functions, i.e.

$$\phi_p(\mathbf{r}) = \sum_{\mu} c_{\mu p} e^{i\mathbf{G}_{\mu} \cdot \mathbf{r}}, \quad (6)$$

where the coefficients  $c_{\mu p}$  are determined through a self consistent solution to the HF equation,  $\mathbf{G}_{\mu}$  is a plane wave vector and  $\mathbf{r}$  is the position of an electron.

Within the Born-Oppenheimer approximation, the orbitals and their energies depend parametrically on the  $n$ th nuclei positions  $\mathbf{R}_n$ , which are not shown in equation 5. Using a plane wave basis, the derivative of the MP2 correlation energy with respect to  $\mathbf{R}_n$  can be expressed concisely as

$$E_{\text{MP2}}^{\text{corr}'} = \frac{\partial E_{\text{MP2}}^{\text{corr}}}{\partial \mathbf{R}_n} = 2 \sum_{pq} P_{pq} F_{pq}', \quad (7)$$

where the prime on quantities refer to their derivatives with respect to  $\mathbf{R}_n$ , the density matrix is defined as a direct sum of the occupied-occupied, unoccupied-unoccupied and occupied-unoccupied blocks

$$P_{pq} = P_{ij} \oplus P_{ab} \oplus P_{ai}, \quad (8)$$

and the derivative on the Fock matrix is

$$F_{pq}' = \sum_{\nu\mu} c_{\nu p} c_{\mu q} h'_{\nu\mu}, \quad (9)$$

where  $h'_{\nu\mu} = \nabla_{\mathbf{R}} \langle \nu | \frac{1}{\mathbf{R}-\mathbf{r}} | \mu \rangle$  can be obtained by taking the derivative in momentum space.

The occupied-occupied and unoccupied-unoccupied blocks of the density matrix can be expressed in closed forms as

$$P_{ij} = - \sum_{abk} t_{ik}^{ab} \frac{\langle jk | ab \rangle}{\varepsilon_i + \varepsilon_k - \varepsilon_a - \varepsilon_b}, \quad (10)$$

$$P_{ab} = \sum_{ijc} t_{ij}^{ac} \frac{\langle ij | bc \rangle}{\varepsilon_i + \varepsilon_j - \varepsilon_b - \varepsilon_c}. \quad (11)$$

While the occupied-unoccupied block, which includes the orbital relaxation effects as we perturb the nuclei coordinates, can be obtained from solving the famous Z-vector equation

$$L''_{ai} - L_{ia} - \sum_{pq} A_{apiq} (P_{ij} + P_{ab}) = (\varepsilon_a - \varepsilon_i) P_{ai} + \sum_{bm} A_{abim} P_{bm}, \quad (12)$$

where the intermediate quantities are defined as

$$L_{ia} = 2 \sum_{cbj} t_{ij}^{cb} \langle cb | aj \rangle, \quad (13)$$

$$L''_{ai} = 2 \sum_{bkj} t_{kj}^{ab} \langle bi | jk \rangle, \quad (14)$$

$$A_{prqs} = 4 \langle pr | qs \rangle - \langle pr | sq \rangle - \langle ps | rq \rangle. \quad (15)$$

An iterative Conjugate Gradient solver is the best suited for solving the Z-vector equation (12) in terms of speed and stability.

Finally, the forces contributed by the MP2 correlation part is

$$\mathbf{F}_{\text{MP2}}^{\text{corr}} = - \frac{\partial E_{\text{MP2}}^{\text{corr}}}{\partial \mathbf{R}} \quad (16)$$

### Implementation Details

Compared to the formulation using nuclei-position dependent Gaussian basis, using plane wave basis simplifies both the theory and implementation. However a relatively large number of plane waves are required to describe the core regions of the wavefunctions that are close to the nuclei, which usually are very oscillatory. To alleviate this problem, we obtain the HF forces within the Projector Augmented Wave (PAW) framework[3, 4], which is implemented in VASP[5], while using pure plane wave basis functions for the MP2 part. We also note that for solid hydrogen systems, it is not so difficult to converge the MP2 forces with respect the number of plane wave basis functions, as we will show shortly. The MP2 analytical gradient has been implemented in CC4S, which uses the **Cyclops Tensor Framework** (CTF)[6] as the backend for massively parallel tensor operations. For the HF part, we sample the 1st Brillouin zone using dense  $k$ -mesh; for the MP2 part, we use only the  $\Gamma$ -point and employ large supercells instead.

### STRUCTURE OPTIMIZATION USING SYMMETRIZED MP2 FORCES

We choose the structures optimized by DFT-PBE forces as our starting point, because they are relatively good approximations to the true stable structures. Since the MP2 forces are much more computationally expansive than the DFT forces, a lot of computational power can be saved by avoiding starting from random structures. On the other hand, since the DFT energy minima are close to the MP2's, a simple gradient descend solver suffices to update the structures and find the most stable MP2 structures. Additionally, due to the numerical noises and other possibly unconverged parameters, the computed forces may not fulfill the space group symmetries which the initial structures have. Therefore, after a few iterations of updating the nuclei positions, the structures can slide into another space group. This is not necessarily a unwanted feature, for example, during random search for the most stable structures, it is perhaps helpful. However we want to focus on the previously found structures and their space groups, because some of them show agreement with experimental spectra studies, indicating that these space groups are promising candidates. So to confine our searches for the most stable structure within a certain space group, we need to symmetrize the computed forces using the corresponding symmetry operations that this space group has.

### Gradient Descend Method

In the gradient descend method, we approximate the energy changes with respect to the changes in the nuclei positions using the first gradient

$$\Delta E = \sum_{\mathbf{n}} \frac{\partial E}{\partial \mathbf{R}_n} \Delta \mathbf{R}_n, \quad (17)$$

and choose the changes in nuclei positions to be

$$\Delta \mathbf{R}_n = -\delta \sum_{\mathbf{n}} \frac{\partial E}{\partial \mathbf{R}_n} = \delta \mathbf{F}_n, \quad (18)$$

where  $\delta$  is a small positive constant which we denote as the time step during the structure optimization procedure. In this case, after we update the nuclei positions, comparing to the previous configuration, the energy is lowered by

$$\Delta E = -\delta \sum_{\mathbf{n}} \left| \frac{\partial E}{\partial \mathbf{R}_n} \right|^2 = -\delta \sum_{\mathbf{n}} |\mathbf{F}_n|^2 < 0. \quad (19)$$

### Symmetrizing the Forces Using Space Group Symmetries

A symmetry is defined as an operation on a system that leaves the system unchanged. A space group element (operation) is a combination of a point group operation (rotation)  $\mathbf{R}$  and a translation operation  $\mathbf{T}$ . Considering a space group which has  $N$  elements, that means we have  $N$  pairs of  $\mathbf{R}$  and  $\mathbf{T}$  operations. Applying one of the element on the coordinates of the nuclei positions  $\{\mathbf{R}_i\}$ , we get

$$\mathbf{R}_i'^n = \mathbf{M}_n \mathbf{R}_i + \mathbf{T}_n, \quad (20)$$

where  $i$  denotes the  $i$ th nuclear position in  $\{\mathbf{R}_i\}$  and  $n$  represents the  $n$ th element from the space group. As per definition of a symmetry operation, we should have two equivalent set of coordinates  $\{\mathbf{R}'\} \equiv \{\mathbf{R}\}$ . Concomitantly, the forces are also transformed by the rotation operation and we use the information from equation (20) to determine the atoms which they act upon. So the transformed forces are

$$\mathbf{F}_i'^n = \mathbf{M}_n \mathbf{F}_i, \quad (21)$$

and the average of forces from all the equivalent atoms resulting from all the operations are the symmetrized forces

$$\bar{\mathbf{F}}_i = \frac{1}{N} \sum_n \mathbf{F}_i'^n. \quad (22)$$

As mentioned before, the HF forces are calculated using the primitive cells and dense  $k$ -meshes, while the MP2 forces are calculated using large supercells and the  $\Gamma$ -point only. To update the coordinates of atoms inside of the primitive cell, a 4-step procedure is carried out

- symmetrizing the MP2 forces using the space group symmetries of the supercell cell;
- downfolding the supercell to the primitive cell by mapping the indices, positions and forces of the atoms between the supercell and the primitive cell;
- symmetrizing the MP2 and HF forces using the space group symmetries of the primitive cell;
- updating the atom positions according to

$$\mathbf{R}_{\text{new}} = \mathbf{R} + \Delta \mathbf{R} = \mathbf{R} + \delta \bar{\mathbf{F}}. \quad (23)$$

### CALCULATION DETAILS AND CONVERGENCE TESTS

In this section we present the details on the calculations carried out, including the parameters used and various convergence tests.

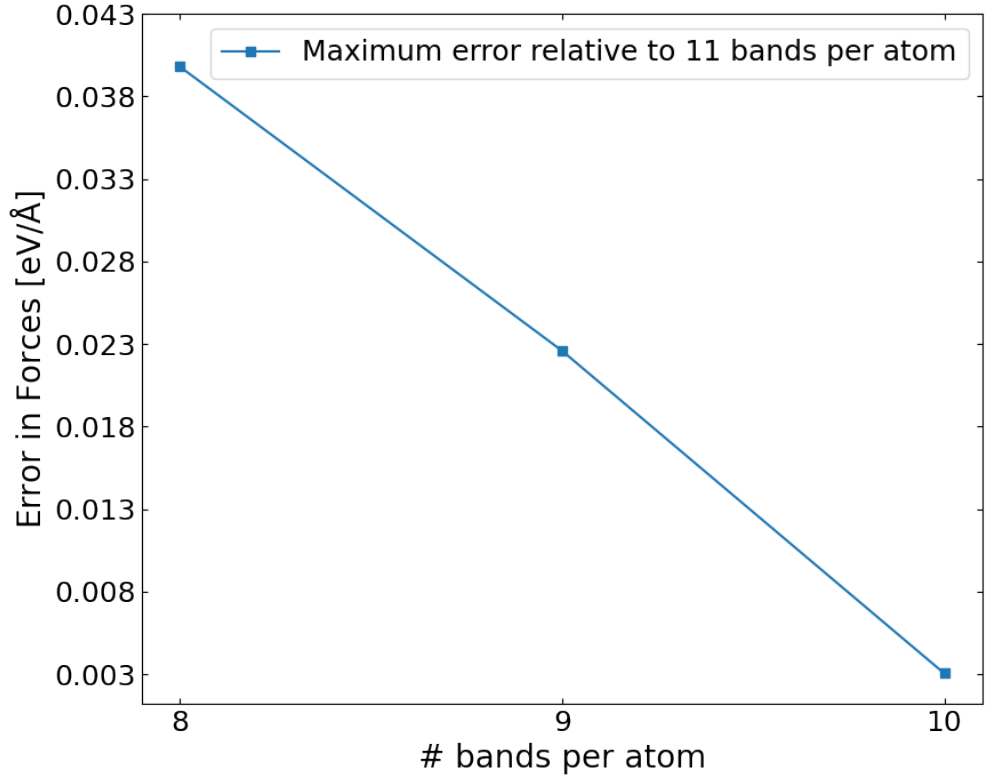

FIG. S1: The maximum error in forces relative to using 11 bands per atom as a function of number of bands.

#### HF and MP2 Forces' convergence with respect to ENCUT

The HF forces are calculated using the PAW pseudopotential with an energy cutoff of 400 eV, which is more than sufficient compared to the VASP officially recommended value of 325 eV (1.3 times of the ENMAX in POTCAR file). A further test using ENCUT=500 eV shows that the maximum error in the HF forces calculated using ENCUT=400 eV is 0.029 eV/Å. The energy cutoff for the plane wave basis in evaluating the orbitals and integrals are both set to 600 eV in the MP2 part. A test carried out at 300 GPa for phase C2/c-24 using 600 eV and 800 eV for the energy cutoffs shows that the MP2 forces are converged to an accuracy of 0.01 eV/Å.

#### MP2 Forces' convergence with respect to number of bands

At 300 GPa, we have tested the convergence of the MP2 forces with respect to the number of bands, using 8, 9, 10 and 11 bands per atom to show that the maximum errors in the forces are well converged to 0.003 eV/Å, see figure (S1)

#### Structural convergence with respect to employed supercell size

The structure optimizations are carried out in two stages. First we employ 4x4x4 k-meshes in sampling the 1st Brillouin zone of the 24-atom primitive cells and only the  $\Gamma$ -point in sampling the 1st Brillouin zone of the 72-atom supercells to get the HF forces and MP2 forces, respectively. Compared to the HF forces evaluated using a  $6 \times 6 \times 6$  k-mesh with all other parameters unchanged, the maximum error in the HF forces is 0.03 eV/Å. After convergence,

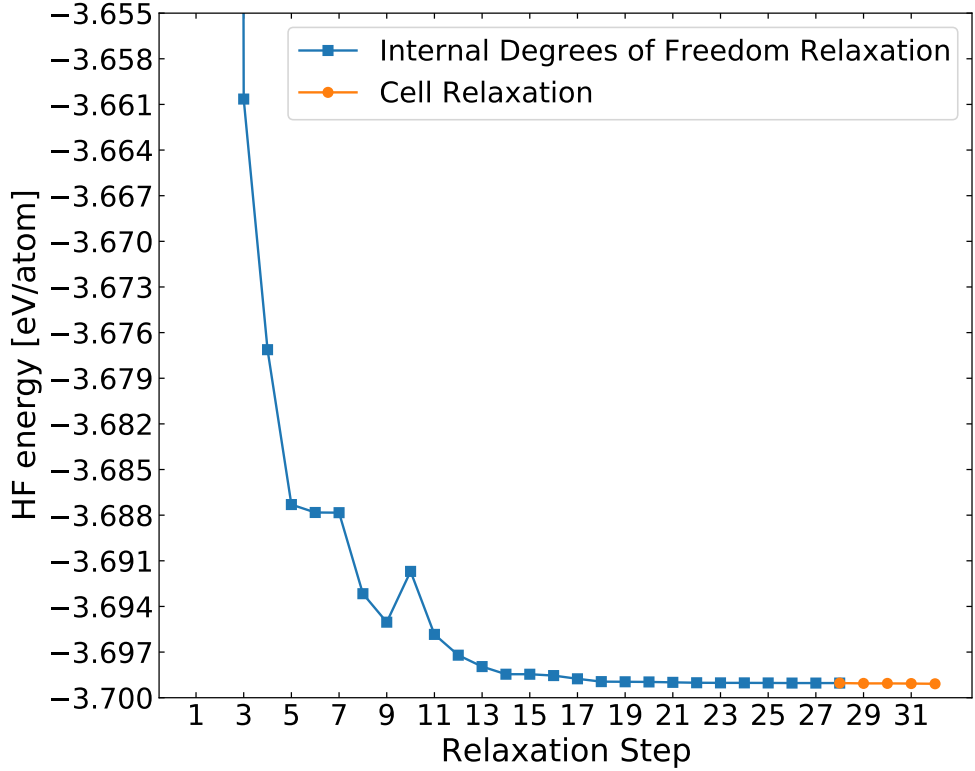

FIG. S2: Two stages of relaxing the C2/c-24 at the DFT pressure 300 GPa using HF forces. On the first stage, the internal degrees of freedom are relaxed, while the cell shape is fixed. During the second stage the cell shape is also allowed to relax. The relaxation of the cell shape has negligible effects on the HF energy.

we increase the  $k$ -meshes in the HF forces step to  $6 \times 6 \times 6$  and the size of supercells to contain 96 atoms. Between these two stages, we found that the total energies per atom are only further lowered by about 2 meV/atom and the gaps are reduced by about 0.27 eV at all pressures. We believe that a further increase in the size of the  $k$ -meshes or the supercell size will not benefit us in terms of the quality of the final result, weighing against the drastic increase in the computational efforts.

### Effects of relaxing the cell shape

Relaxing the cell shapes on the MP2 level would require the calculation of the stress tensor, which at the current stage is not implemented. However the effects of relaxing the cell parameters can be estimated using the HF forces and stress tensors. To this end, we first relax the internal degrees of freedom of the PBE structures while keeping the cell parameters fixed and on the second stage we also allow the latter to change. By observing how the HF energy is further lowered during the second stage, we can estimate the impact of the relaxed cell shape.

The above procedure is carried out on the DFT-PBE C2/c-24 structure at 300 GPa, using a  $5 \times 5 \times 5$   $k$ -mesh sampling the 1st BZ and an energy cutoff of 400 eV along with PAW potential. Between the first and second step, the HF energy is lowered by 0.0011 eV in total (0.000047 eV/atom), see figure (S2).

# Electron-phonon interactions

Electron-phonon interactions (EPIs) were considered by combining QUANTUM ESPRESSO (QE) [7] and YAMBO [8]. In the QE calculations, the DFT ground state were obtained using ONCVSP (Optimized Norm-Conserving Vanderbilt Pseudopotential) pseudopotential file [9] with a kinetic energy cutoff at 100 Ry and a uniform  $4 \times 4 \times 4$   $k$ -grid. In the YAMBO calculations, the electron-phonon self-energies were obtained using 100 random  $q$ -points in the phonon Brillouin zone, a uniform  $4 \times 4 \times 4$   $k$ -grid for electronic Brillouin zone and 300 electronic bands. The convergence tests are given as follows.

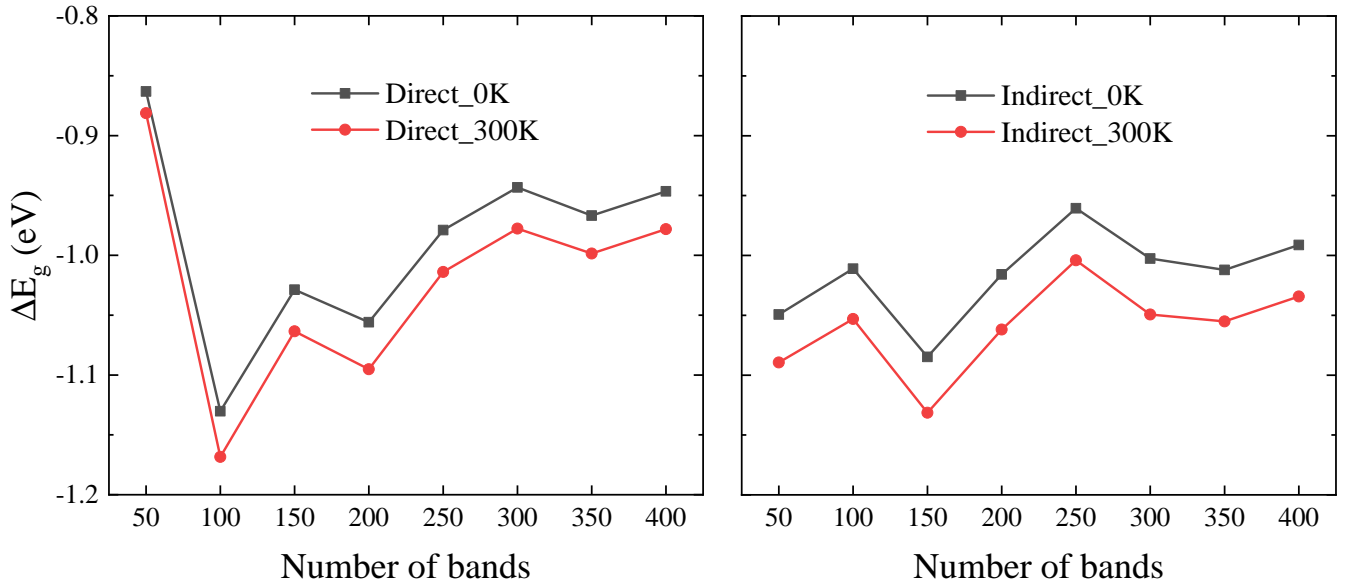

FIG. S3: The convergence test of the direct (black) and indirect (red) band gaps renormalization as a function of the number of electronic bands at 0 K and 300 K, respectively. The structure is model phase III (C2/c-24) obtained using DFT-PBE at 250 GPa. 5 random  $q$ -points and  $4 \times 4 \times 4$   $k$ -grid are used.

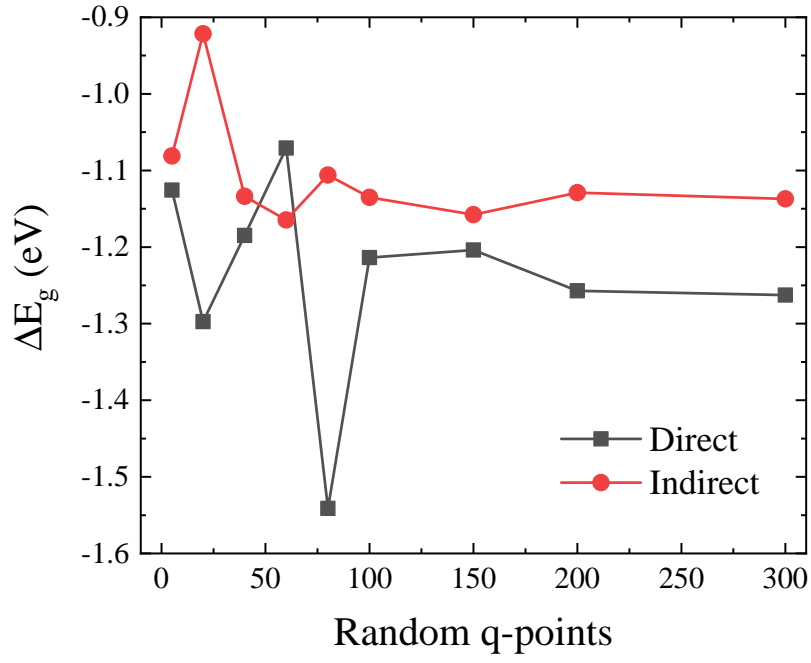

FIG. S4: The convergence test of the direct (black) and indirect (red) band gaps renormalization as a function of the number of random q-points. The structure is model phase III (C2/c-24) obtained using DFT-PBE at 250 GPa. The number of electronic bands is 64 and  $4 \times 4 \times 4$   $k$ -grid is used.

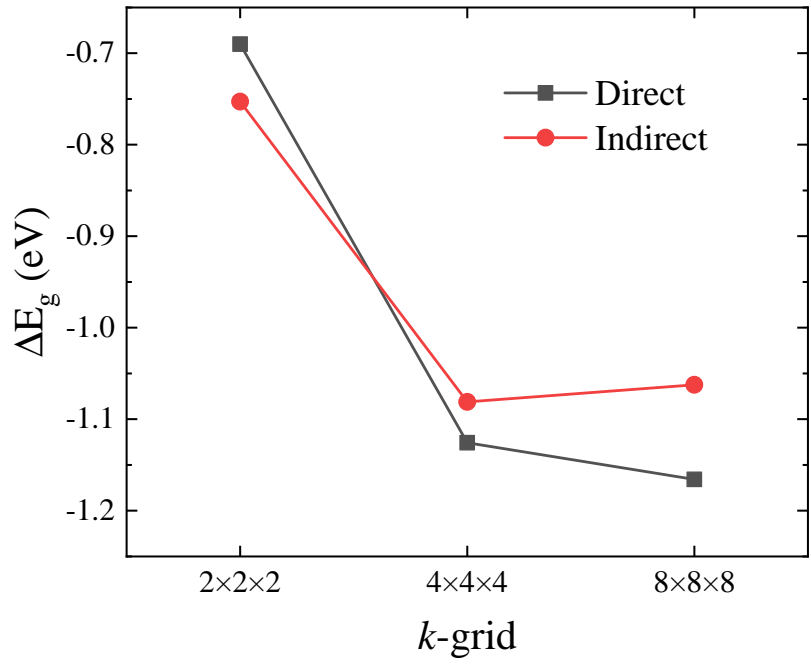

FIG. S5: The convergence test of the direct (black) and indirect (red) band gaps renormalization as a function of the number of  $k$ -points. The structure is model phase III (C2/c-24) obtained using DFT-PBE at 250 GPa. 5 random q-points and 64 electronic bands are used.

### $T$ -dependent band gap renormalization

The  $T$  dependence of band gap is shown in Fig. S6. As we can see, the difference of  $T$ -dependent indirect band gap renormalizations at 300 GPa between 100 K and 300 K is only 24 meV, which is in great agreement with experimental data [? ? ].

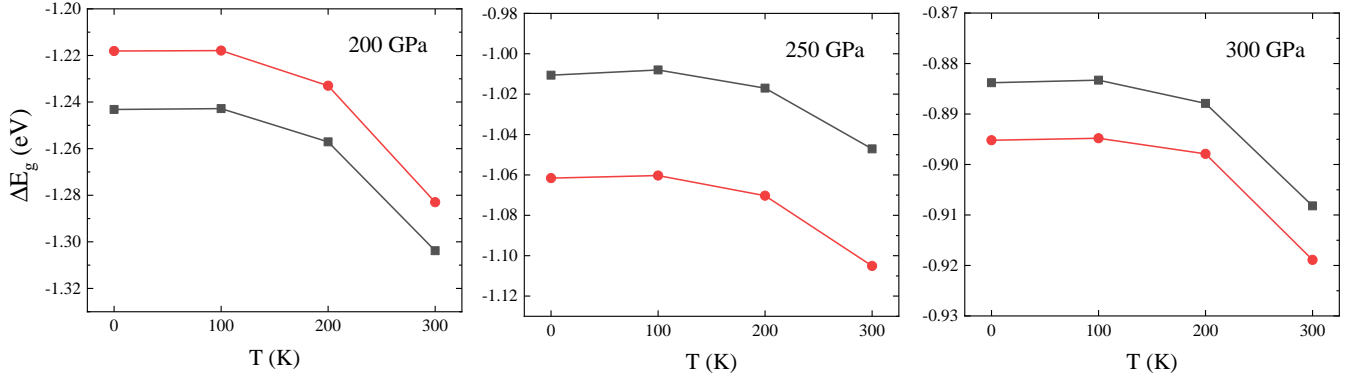

FIG. S6:  $T$ -dependent direct (black squares) and indirect band gaps (red circles) of model phase III (C2/c-24) obtained using DFT-PBE at 200, 250 and 300 GPa, calculated using dynamical HAC theory. 100 random q-points, 300 electronic bands and a  $4 \times 4 \times 4$   $k$ -grid are used.

### Exciton binding energy

The electron-hole interactions were obtained using Vienna *ab initio* simulation package (VASP) in solving Bethe-Salpeter equation (BSE). 800 eV energy cutoff and 96 electronic bands are used. A dense uniform  $4 \times 4 \times 4$   $k$ -grid is necessary to converge the oscillator strength (see Fig. S7).

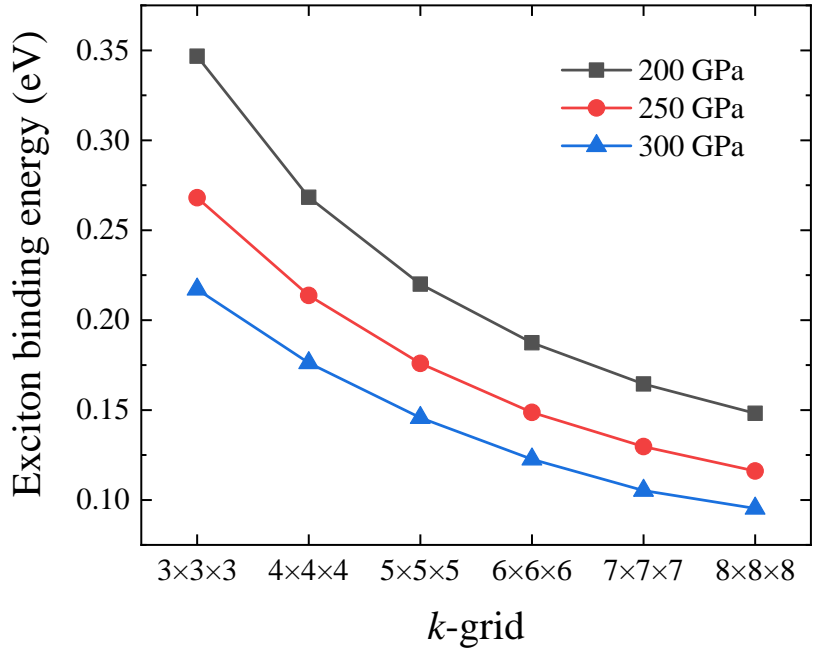

FIG. S7: The convergence tests of the exciton binding energy as a function of the number of  $k$ -grid. The structure is model phase III (C2/c-24) obtained using DFT-PBE at 200, 250 and 300 GPa, respectively.

- 
- [1] M. Del Ben, J. Hutter, and J. VandeVondele, *The Journal of Chemical Physics* **143**, 102803 (2015).
  - [2] F. Weigend and M. Hser, *Theoretical Chemistry Accounts* **97**, 331 (1997).
  - [3] G. Kresse and D. Joubert, *Physical Review B* **59**, 1758 (1999).
  - [4] P. E. Blöchl, *Phys. Rev. B* **50**, 17953 (1994).
  - [5] G. Kresse and J. Furthmüller, *Phys. Rev. B* **54**, 11169 (1996), iSBN: 1098-0121.
  - [6] E. Solomonik, D. Matthews, J. R. Hammond, J. F. Stanton, and J. Demmel, *Journal of Parallel and Distributed Computing* **74**, 3176 (2014), publisher: Academic Press.
  - [7] P. Giannozzi, S. Baroni, N. Bonini, M. Calandra, R. Car, C. Cavazzoni, D. Ceresoli, G. L. Chiarotti, M. Cococcioni, I. Dabo, and A. Dal Corso, *J. Phys. Condens. Matter* **21**, 395502 (2009).
  - [8] D. Sangalli, A. Ferretti, H. Miranda, C. Attaccalite, I. Marri, E. Cannuccia, P. Melo, M. Marsili, F. Paleari, A. Marrazzo, G. Prandini, P. Bonfa, M. O. Atambo, F. Affinito, M. Palumbo, A. Molina-Sanchez, C. Hogan, M. Gruning, D. Varsano, and A. Marini, *J. Phys.: Condens. Matter* **31**, 325902 (2019).
  - [9] D. Hamann, *Physical Review B* **88**, 085117 (2013).
  - [10] V. Gorelov, M. Holzmann, D. M. Ceperley, and C. Pierleoni, *Physical Review Letters* **124** (2020), 10.1103/physrevlett.124.116401.
